# Supplementary material for: The AI Ghostwriter Effect: When Users Do Not Perceive Ownership of AI-Generated Text But Self-Declare as Authors
Source: arXiv:2303.03283 source file (2023-11-07)
Supplement: Supplementary file 1 [file Non-Personalized_Generated_Texts.pdf]

# Non-Personalized Generated Texts

## Set 1

### Editing

Hey Friend, I'm in New York and it's amazing! I'm staying in a really great hotel in the heart of the city and I've been doing a lot of sightseeing. I've been to the top of the Empire State Building, Central Park, and a bunch of other places. The city is so big and there's so much to do! I'm really enjoying myself. I wish you were here with me! We would have so much fun exploring everything together. But I'm glad you're getting to experience your own adventures. I can't wait to hear all about them when I get back home. I hope you're doing well and I miss you! [Your Name]

### Choosing - Text 1

Dear Friend, I hope you're doing well! I'm having a great time in New York. The city is huge and there's so much to do. I've been walking around a lot and exploring. Yesterday, I went to the top of the Empire State Building and it was incredible. You could see for miles. I also went to Central Park, which was really pretty. I have attached a picture of me in front of the fountain. I'm really enjoying my time here and I can't wait to show you everything when you come visit. Hope to hear from you soon, [Your Name]

### Choosing - Text 2

Hey there! I'm currently in the middle of a whirlwind trip to New York and I'm having an absolute blast! The city is so alive and there is so much to see and do. I started my trip with a walk through Central Park, which was gorgeous. I then went and did some shopping on Fifth Avenue, which was a lot of fun. I also made sure to visit the Empire State Building and the Statue of Liberty, which were both incredible. I'm currently staying in a great hotel in the heart of the city and I'm just loving every minute of my time here. I really wish you were here with me so we could enjoy all of this together. I'm just having the best time and I can't wait to come back and visit again. In the meantime, I'll be sure to send you lots of pictures so you can see what I'm up to. Hope to talk to you soon, [Your Name]

### Choosing - Text 3

Dear Friend, I hope you're doing well! I'm having a great time in New York. The city is so big and there's so much to see and do. I've been to a lot of great restaurants and seen some amazing shows. I'm really enjoying myself. I'm staying in a great hotel in the middle of the city. It's really close to everything, which is great. I've been walking a lot and taking the subway to get around. It's been a lot of fun. I'm really enjoying my time here and I can't wait to explore more of the city. I'm already planning my next trip. I hope you can come visit me soon. I'll show you around. Take care, [Your name]

## Getting

Dear Friend, Greetings from New York City! I hope all is well with you and that you're enjoying your summer. I'm having a great time here in the Big Apple. The weather has been really nice lately, so I've been spending a lot of time outdoors. I've been doing a lot of exploring since I got here. I've walked across the Brooklyn Bridge, visited the top of the Empire State Building, and strolled through Central Park. I've also been to a few museums, including the Metropolitan Museum of Art and the Museum of Natural History. I could spend days in those places and still not see everything! The city is so exciting and there's always something new to do. I can't wait to see what else the next few weeks have in store. I'm sure I'll have plenty more to tell you when I get home. Hope to hear from you soon, [Your Name]

## Set 2

### Editing

My dear friend, Greetings from New York! I hope all is well with you. I'm having a wonderful time here in the Big Apple. The city is so vibrant and alive. There's so much to see and do. I've been keeping busy sightseeing and exploring. I've been to the top of the Empire State Building, Rockefeller Center, Central Park, and the Statue of Liberty. I've also done a lot of shopping. The stores here are amazing. I've bought so many new clothes and shoes. I can't wait to show you everything when I get home. I'm also enjoying the food here. I've had some of the best meals of my life. The other night I had dinner at a fancy restaurant. The food was incredible. I'm really going to miss the food here when I go home. I miss you and can't wait to see you. I'll be home in a few weeks. I can't wait to tell you all about my adventure. Love, Your friend

### Choosing - Text 1

Dear Friend, I hope this postcard finds you well! I'm having a great time in New York. The city is so big and there's so much to do. I've been to a few museums, Central Park, and a few Broadway shows. I'm really enjoying myself. I'm staying in a great hotel in Times Square. It's so busy and lively here. I'm never bored. I'm sorry I couldn't be there for your birthday, but I'll make it up to you when I get home. I hope you're doing well. I miss you and can't wait to see you soon. Love, Your friend

### Choosing - Text 2

Dear Friend, I hope you're doing well! I'm having a great time in New York City. It's been really fun exploring all the different neighborhoods and finding new things to do. I've been going to a lot of museums, and the other day I went to the top of the Empire State Building. The views from up there are incredible. I also went to a Broadway show, which was really great. I'm really enjoying the food here too. There are so many different restaurants and cafes to choose from. I've been trying a lot of new things, and I'm really liking it. I think my favorite thing so far has been the pizza. It's so good! I'm attaching a few pictures from my trips around the city. I hope you have a chance to come visit soon. I think you would really like it here. Take care, [Your name]

## Choosing - Text 3

Dear Friend, I hope you're doing well! I'm currently in New York and absolutely loving it! The city is so vibrant and there's always something to do. I've been exploring a lot and trying new things. Just last week, I went to my first Broadway show and it was amazing! I'm also planning on seeing a few more shows while I'm here. I've been doing a lot of walking around and exploring different neighborhoods. I love how each neighborhood has its own personality. I've also been eating a lot of great food. There's so much to choose from and I've been trying to get a little bit of everything. I'm having a great time and can't wait to explore more of this amazing city. I hope to see you soon!

## Getting

Dear Friend, I hope this postcard finds you well! I'm having a great time in New York – the city is truly amazing. There's so much to see and do here, and I feel like I'm barely scratching the surface. I've been doing a lot of walking around and exploring different neighborhoods, and I've already eaten my way through a lot of the great restaurants here. I'm really looking forward to seeing more of the city and checking out some of the famous tourist attractions. The weather has been perfect – sunny and warm, with a cool breeze. I've been taking advantage of the nice weather by spending time outdoors, whether it's walking around or just relaxing in one of the many parks here. Central Park is my favorite so far, but I'm looking forward to exploring more of the city's green spaces. I miss you and can't wait to catch up when I get back, but in the meantime, I hope you're doing well and enjoying your summer. Take care, [Your Name]

## Set 3

## Editing

Dear Friend, I hope this postcard finds you well! I'm currently in New York and loving it! The city is so vibrant and alive - there's always something to do, no matter what time of day or night it is. I've been here for a week now and I feel like I've barely scratched the surface of all there is to see and do. So far, some of my favorite experiences have been exploring Central Park, taking in the views from the top of the Empire State Building, and spending an afternoon walking around Greenwich Village. I'm also a big fan of the food here - I've had some amazing meals since I arrived! If you ever have the opportunity to come to New York, I would highly recommend it. I think you would love it as much as I do! Hope to hear from you soon, [Your name]

## Choosing - Text 1

Dear Friend, I hope this postcard finds you well! I'm having a great time in New York. The city is so big and there's so much to do. I've been to a few museums, Central Park, and a few Broadway shows. I'm really enjoying myself. I'm staying in a great hotel in Times Square. It's so busy and lively here. I'm never bored. I'm sorry I couldn't be there for your birthday, but I'll make it up to you when I get home. I hope you're doing well. I miss you and can't wait to see you soon. Love, Your friend

## Choosing - Text 2

Hey there! I'm loving New York so far! The city is huge and there's so much to do. I haven't been here long, but I've already walked around Central Park, gone to the top of the Empire State Building, and seen a Broadway show. The people here are really friendly too. I was struggling to find my way to the subway the other day and this guy helped me out. He ended up being my tour guide for the day and showed me some of the best places to eat and shop. I can't wait to explore more of this amazing city. I'm sure I'll never get tired of it. Thanks for letting me share my adventure with you! Love, your friend

## Choosing - Text 3

Dear Friend, Greetings from New York! It's been a while since we've seen each other and I'm sure you're wondering what I've been up to. Well, let me tell you, it's been quite a ride. I moved to New York about a year ago now, and it's been everything I hoped for and more. The city is always alive, there's always something new to see and do. I've made some great friends here, and we always seem to find ourselves in the most interesting situations. I'm really loving my life here, and I think you would too. If you ever have the chance, you should definitely come and visit me. I'll show you around my city and we can have the time of our lives. I'll be waiting for your visit! Love, your friend

## Getting

My dear friend, I hope this postcard finds you well! I am currently in New York and let me tell you, it is quite the experience. The hustle and bustle of the city is unlike anything I've ever seen before. Everywhere you look, there's something new to see. I've been here for a few days now and I'm still not sure I've seen it all. One of the best parts of New York, in my opinion, is the food. You can find just about anything here, no matter what your taste. I've already tried a few of the local specialties and they were all delicious. I can't wait to try more. I'm also enjoying the nightlife here. There's always something going on, no matter what time of day or night it is. It's really unlike anywhere else I've ever been. All in all, I'm having a great time here in New York. I can't wait to explore more of this amazing city. I'm sure you would love it here too. Until next time, Your friend
